# Supplementary material for: An Extensive Study of User Identification via Eye Movements across Multiple Datasets
Source: arXiv:2111.05901 source file (2021-11-10)
Supplement: Supplementary file 1 [file Appendix.tex]

\section{Appendix}
\subsection{User Identification}
%\subsection{User prediction with Bioeye Dataset}
\label{comparsion_user_prediction}

\begin{table}[!ht]
	\caption{The velocity threshold against the highest number of fixation over all the participants in session one,  prediction accuracy of using 51 features and over 50 runs in all the data sets (except for VST, 10 runs are used in this experiment).}
	\label{table_ivt_parameters}
	\begingroup
	\setlength{\tabcolsep}{1.4pt} % horzontal distance Default value: 6pt
	 % vertical distance Default value: 1
	\begin{tabular}{ccc|ccc}
		%		\centering
		\toprule
		& RAN & & & TEX &\\
		\midrule
		Vel. & Fix. No. & Acc.\,\% &Vel. &  Fix. No.& Acc.\,\%  \\
		threshold & & & threshold &  &  \\
		\midrule
		23 &31959&94.27&23&33515& 92.25 \\
		\bf{24} &\bf{31961}&94.89&24&33520&92.48\\
		25 &31933&94.93&25&33540&92.65\\
		26 &31889&94.86&\bf{26}&33584&\bf{93.23}\\
		\bf{27} &31779&\bf{95.96}&27&33597&92.65\\
		28 &31700&95.03& 28 &33594&92.56 \\
		29 &31582&94.91& 29 &33617&92.31\\
		30 &31490&95.20&\bf{30}&\bf{33623}&92.24\\
		31 &31355&94.56& 31 &33617&92.86\\
		32 &31255&94.71& 32 &33602&92.84 \\				
		\toprule
		& VST data & &  & GOF data &  \\
		\midrule
		Vel. & Fix. No. & Acc.\,\% &Vel. &  Fix. No.& Acc.\,\%  \\
		threshold & & & threshold &  &  \\
		\midrule
		80 & 24987 &93.10&   16 &52514 & 80.51\\
		90 & 27883 &93.27&   17 &54289 & 80.83\\
		\bf{100} & 29818 &\bf{94.82}& 18 &  55399 & 81.56\\
		110 & 30715 &94.80&19 &  56065 & 82.19\\
		\bf{120}&\bf{31021}&94.31&20 &  56408& 82.51\\
		130 & 30684 &92.84 &\bf{21}&\bf{56490}& 82.35\\
		140 & 30077 &94.48&\bf{22}&  56391 &\bf{83.45}\\
		150 &29180 &94.30 & 23 & 56079 & 83.25\\
		160 & 28307&94.27 & 24 & 55701 & 83.40\\
		170 & 27419&91.72&25 & 55268 & 83.23\\
		\bottomrule
	\end{tabular}
	\endgroup
\end{table}

\begin{table}[!ht]
	\caption{Variation of MFD against the accuracy of user identification over 122 participants 50 runs in BioEye dataset. (VT is fixed to 27 °/s)}
	\label{Varying_MDF_and_fixing_VT}
	\begingroup
	\setlength{\tabcolsep}{1.4pt} % horzontal distance Default value: 6pt
	 % vertical distance Default value: 1
	\begin{tabular}{ccc|ccc}
		%		\centering
		\toprule
		& RAN & & & TEX &\\
		\midrule
		Vel. & MFD & Acc.\,\% &Vel. & MFD & Acc.\,\%  \\
		threshold & & & threshold &  &  \\
		\midrule
		27& 0.05 &94.62 & 26 & 0.05 &93.13\\
		27& 0.06&94.63 & 26 & 0.06 &93.18 \\
		27& 0.07&95.03 & 26 & 0.07 &93.26\\
		27&0.08&95.73 & 26 & 0.08 & 93.31\\
		27& 0.09&95.57& 26 & 0.09 &93.44\\
		27&\bf{0.095}&\bf{96.14}& 26 & 0.095 &93.73\\
		27&\bf{0.096}&\bf{96.14}&26 & 0.096 & 93.73\\
		27&\bf{0.097}&\bf{96.09}&26 &\bf{0.097} &\bf{94.18}\\
		27&\bf{0.098}&\bf{96.09}&26 &\bf{0.098} &\bf{94.18}\\
		27&\bf{0.099}&\bf{96.09}& 26 &\bf{0.099} &\bf{94.18} \\
		27&\bf{0.1}&\bf{96.09}&26 &\bf{0.1} &\bf{94.18} \\
		27&\bf{0.101}&\bf{96.04}& 26 & 0.101 & 93.73\\
		27&\bf{0.102}&\bf{96.04}& 26 & 0.102 & 93.73 \\
		27&\bf{0.103}&\bf{96.04}& 26 & 0.103 &93.73  \\
		27&\bf{0.104}&\bf{96.04}& 26 & 0.104 &93.73 \\
		27&0.105&95.98 & 26 & 0.105 &93.42  \\
		27&0.11&95.09 & 26 & 0.11 &93.34  \\
		27&0.12&94.70 & 26 & 0.12 &93.19 \\
		27&0.13&93.83 & 26 & 0.13 &92.44  \\
		27&0.14&94.13 & 26 & 0.14 &91.68 \\
		27&0.15&93.72& 26 & 0.15 &91.01  \\	
		\bottomrule
	\end{tabular}
	\endgroup
\end{table}
